# Supplementary material for: Shear-layer effects on the dynamics of unsteady premixed laminar counterflow flames
Source: arXiv:2510.25109 ancillary file (2025-10-29)
Supplement: Supplementary file 1 [file Suppl_file_Rivera-Lizarralde_et_al.pdf]

# Supplementary materials: Shear-layer effects on the dynamics of unsteady premixed laminar counterflow flames

Jose G. Rivera Lizarralde, Aditya Potnis, Abhishek Saha

University of California San Diego

This document contains supporting information and additional data from experiments presented in the manuscript titled above.

## 1 Additional data for *constant amplitude*

In this section, we present additional figures for the *constant amplitude* method.

### 1.1 Time series of flame oscillation:

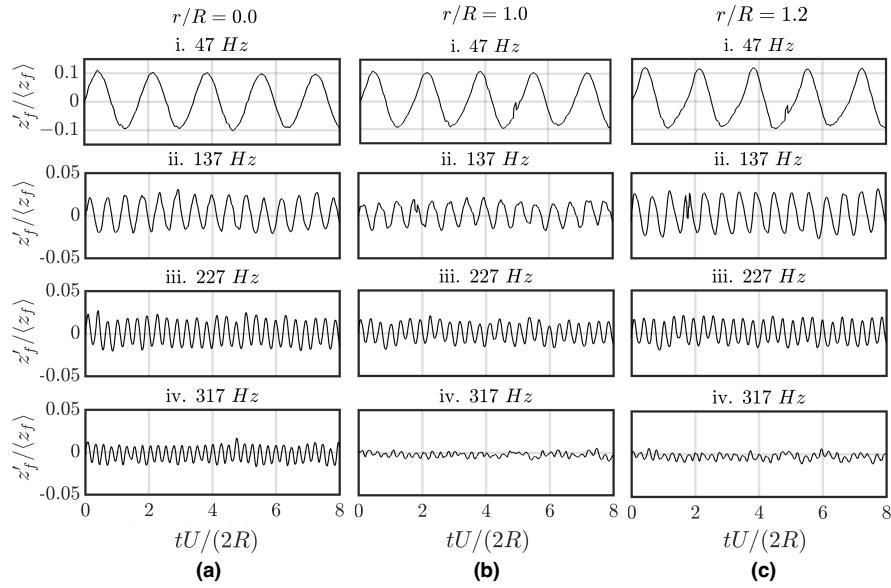

Figure 1: Normalized prime flame displacement signals measured at (a) flame's center point ( $r/R = 0$ ), (b) flame location  $r/R = 1.0$ , and (c) flame location  $r/R = 1.2$  at different excitation frequencies (i-iv.).

We start by displaying the local time series of flame oscillation at both center and off-center locations. Figure 1(a-c) presents the time series of the flame displacement fluctuations normalized with the mean flame location ( $z'_f / \langle z_f \rangle$ ) at three radial locations: the centerline ( $r/R = 0$ ), and two off-center positions ( $r/R = 1.0$ , and  $r/R = 1.2$ ), for all four excitation frequencies. At the centerline, the time series clearly exhibits a single-frequency sinusoidal behavior. As we move away from the center, the flame response exhibits increasingly multi-frequency behavior. This is caused by the emergence of higher harmonics at integer multiples of the excitation frequency.

## 1.2 Other stretch rates:

Next, we show the data for two stretch rates that are not discussed in the manuscript. Figures 2(a-c) and 4(a-c) show the power spectral density (PSD) of  $\hat{P}_{K_n}$  and  $\hat{P}_{K_c}$ , at three radial locations: the centerline ( $r/R = 0$ ), and two off-center positions ( $r/R = 1.0$ , and  $r/R = 1.2$ ), for all four excitation frequencies. Figures 2(d) and 4(d) compare the radial distribution of the spectral energy at the excitation frequency and its higher harmonics for the different excitation cases. We also extracted the radial profiles of the mean and RMS of these stretch rates, shown in Fig. 3 and 5. Clearly, PSDs, mean, and RMS of  $K_n$  and  $K_c$  bear a strong resemblance to the PSD of flame oscillations and  $K_t$  shown in the main manuscript.

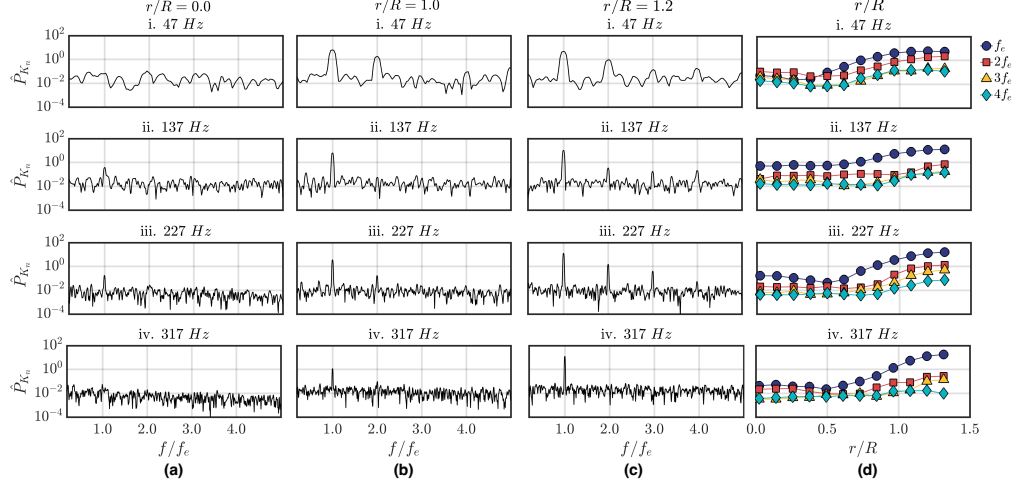

Figure 2: Power spectral density of flame conditioned stretch rate due to normal strain ( $\hat{P}_{K_n}$ ) measured at (a) flame's center point ( $r/R = 0$ ), (b) flame location  $r/R = 1.0$ , and (c) flame location  $r/R = 1.2$  accompanied by (d) radial profiles of first four harmonics of the  $\hat{P}_{K_n}$  (markers are displayed every 6 data points for clarity). Four rows represent four excitation frequencies: (i.) 47 Hz, (ii.) 137 Hz, (iii.) 227 Hz, and (iv.) 317 Hz.

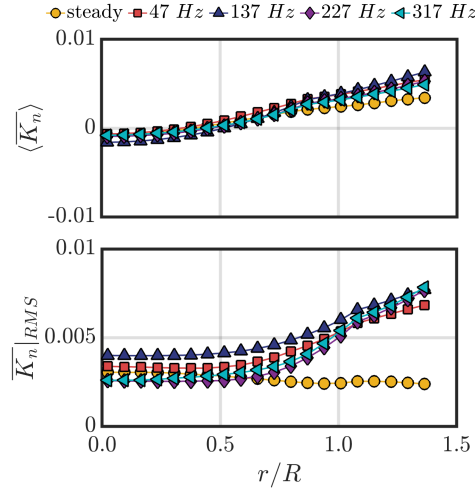

Figure 3: Radial profiles of mean and root-mean-square of normalized stretch rate due to normal strain,  $\overline{K_n}$ , at different excitation frequencies and for steady case (markers are displayed every 3 data points for clarity).

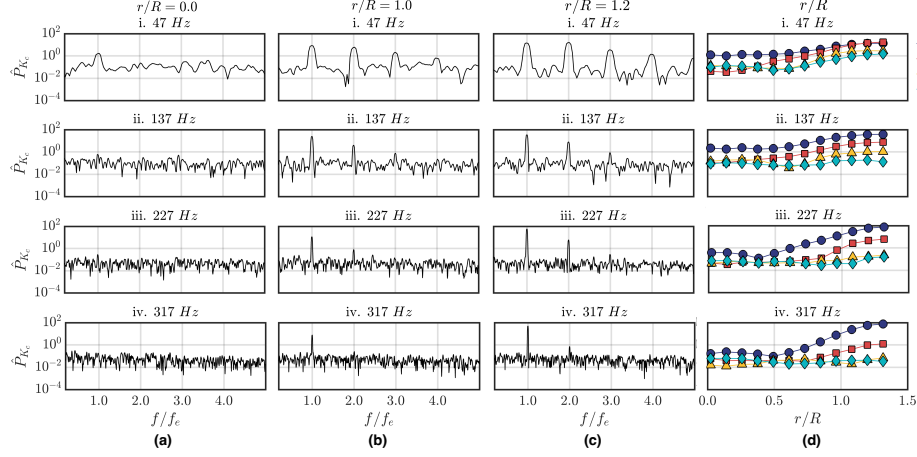

Figure 4: Power spectral density of flame conditioned stretch rate due to curvature ( $\hat{P}_{K_c}$ ) measured at (a) flame's center point ( $r/R = 0$ ), (b) flame location  $r/R = 1.0$ , and (c) flame location  $r/R = 1.2$  accompanied by (d) radial profiles of first four harmonics of the  $\hat{P}_{K_c}$  (markers are displayed every 6 data points for clarity). Four rows represent four excitation frequencies: (i.) 47 Hz, (ii.) 137 Hz, (iii.) 227 Hz, and (iv.) 317 Hz.

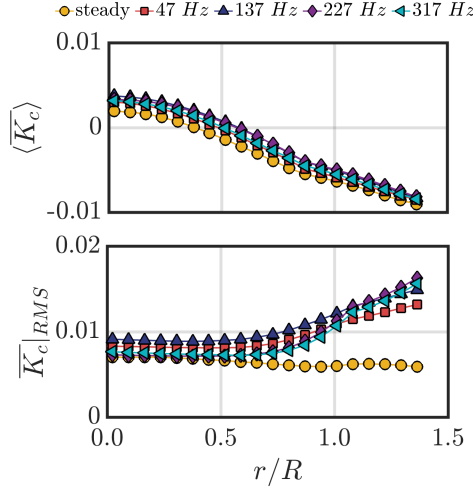

Figure 5: Radial profiles of mean and root-mean-square of normalized stretch rate due to curvature,  $\overline{K_c}$ , at different excitation frequencies and for steady case (markers are displayed every 3 data points for clarity).

### 1.3 Phase-averaged vorticity

Next, we portray the phase-averaged vorticity field in Fig. 6 for  $f_e = 47$  Hz,  $f_e = 227$  Hz, and  $f_e = 317$  Hz. These phase-averaged snapshots spanning from  $\phi = 0^+$  to  $\phi = 2\pi^-$  reveal the real-time evolution and advection of the vortices along the shear layer. The sequence clearly shows the formation and advection of the pair of counter-rotating vortices ( $A_1$  and  $B_1$  in the figure) along the shear layer during the cycle, and their eventual approach towards the outer edge of the flame.

To extract the phase-averaged dynamics of the flow, we employed a Hilbert transform-based phase reconstruction of the velocity signal at a representative probe location ( $r/R = 0$ ,  $z/H = 1.0$ ). Specifically, a single velocity time series was selected from the two-dimensional velocity field, the mean was subtracted, and normalized. The analytic signal was then computed using the Hilbert transform, and the instantaneous phase was obtained from the unwrapped argument of the complex signal. Zero crossings of the normalized time series were used to count oscillation cycles, and for each cycle the phase was discretized into 32 uniformly spaced intervals ( $\pi/16$  increments). For every target phase value within each cycle, the closest time index was identified, thereby constructing an index set of snapshots corresponding to evenly spaced phases across multiple oscillations. The corresponding instantaneous

velocity and vorticity fields were then collected at these indices, and the phase-averaged quantities were computed by ensemble-averaging across cycles.

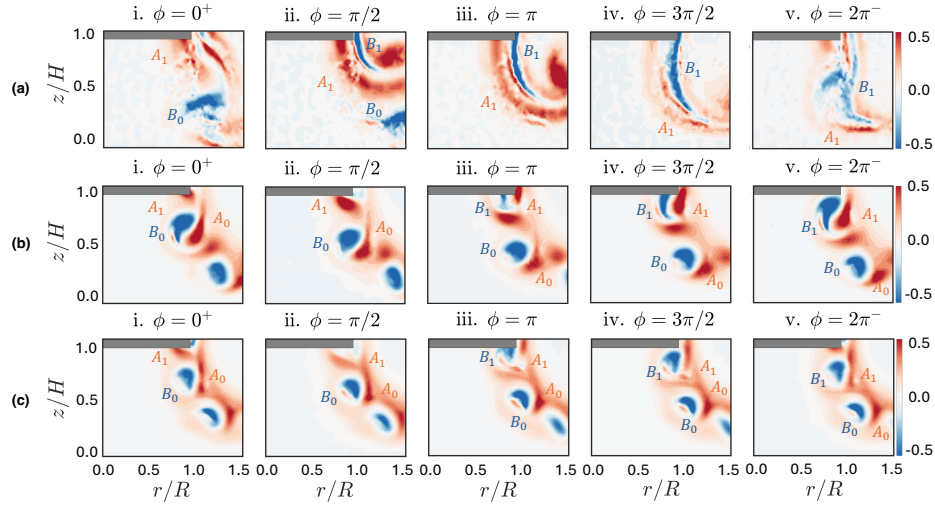

Figure 6: Phase-averaged vorticity for one excitation cycle for (a)  $f_e = 47$  Hz, (b)  $f_e = 227$  Hz, and (c)  $f_e = 317$  Hz at five phase angles from  $0^+$  to  $2\pi^-$  (i.-v.). The schematic represents the top-right quadrant corner of the counterflow. A and B are large counter-rotating vortex pairs generated during each cycle. Subscripts 0, 1, and 2 refer to vortices originating from the previous, current, and next cycle, respectively.



## 2 Additional data for *constant power*

In this section, we present the data associated with the *constant power* method, illustrating dynamics similar to those of the *constant amplitude* method.

### 2.1 Flame oscillation

We start by discussing the local spectral signature of flame oscillation at both center and off-center locations. Figure 7(a-c) presents the PSDs of the flame displacement ( $\hat{P}_{z_f}$ ) at three radial locations: the centerline ( $r/R = 0$ ), and two off-center positions ( $r/R = 1.0$ , and  $r/R = 1.2$ ), for all four excitation frequencies.

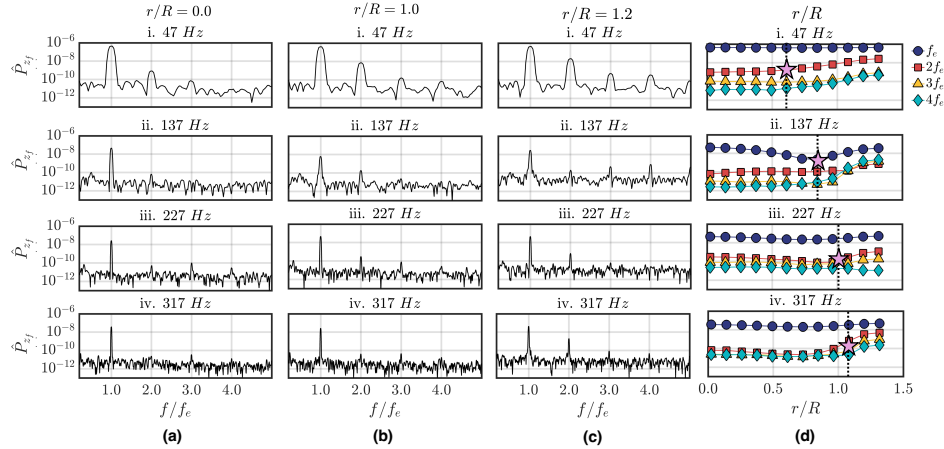

Figure 7: Power spectral density of flame oscillation or displacement ( $\hat{P}_{z_f}$ ) measured at (a) flame's center point ( $r/R = 0$ ), (b) flame location  $r/R = 1.0$ , and (c) flame location  $r/R = 1.2$  accompanied by (d) radial profiles of first four harmonics of the  $\hat{P}_{z_f}$  of *constant power* method (markers are displayed every 6 data points for clarity). The radial location ( $r_{2f_e}$ ) where  $2f_e$  starts to increase is marked with a star and a vertical dashed line in (d). Four rows represent four excitation frequencies: (i.) 47 Hz, (ii.) 137 Hz, (iii.) 227 Hz, and (iv.) 317 Hz. The uncertainty in the computation of  $z_f$  is  $\pm 2$  pixel.

### 2.2 Stretch rate due to the tangential strain rate

Figure 8(a-c) shows the power spectral density of flame conditioned stretch rate due to tangential strain,  $\hat{P}_{K_t}$ , at three radial locations: the centerline ( $r/R = 0$ ), and two off-center positions ( $r/R = 1.0$ , and  $r/R = 1.2$ ), for all four excitation frequencies. Figure 8(d) compares the radial distribution of the spectral energy at the excitation frequency and its higher harmonics for the different excitation cases. We have also extracted the radial profiles of the mean,  $\langle \bar{K}_t \rangle$ , and RMS of the fluctuations,  $\bar{K}_t|_{RMS}$  for the normalized stretch rate due to tangential strain ( $\bar{K}_t = K_{ttf}$ ) under four excitation frequencies and compare them with the steady condition in Fig. 9.

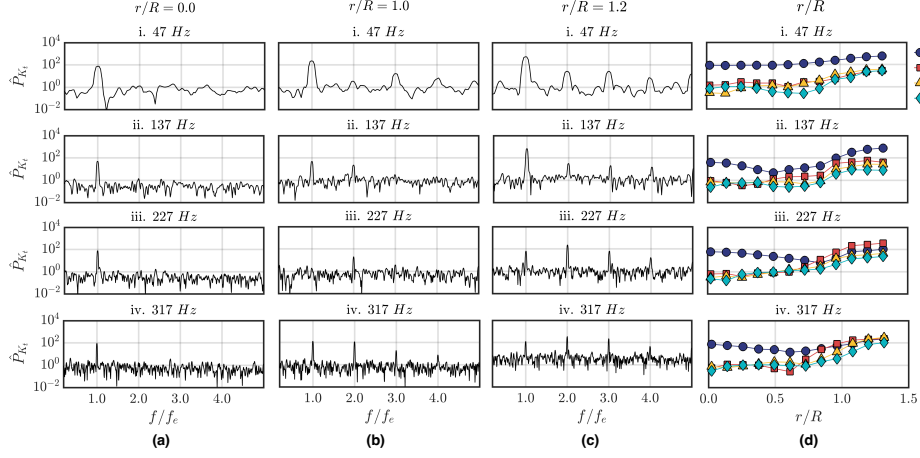

Figure 8: Power spectral density of flame conditioned stretch rate due to tangential strain ( $\hat{P}_{K_t}$ ) measured at (a) flame's center point ( $r/R = 0$ ), (b) flame location  $r/R = 1.0$ , and (c) flame location  $r/R = 1.2$  accompanied by (d) radial profiles of first four harmonics of the  $\hat{P}_{K_t}$  of *constant power* method (markers are displayed every 6 data points for clarity). Four rows represent four excitation frequencies: (i.) 47 Hz, (ii.) 137 Hz, (iii.) 227 Hz, and (iv.) 317 Hz. The uncertainty in the computation of  $\overline{K_t}$  is  $0.01 - 0.02$  1/s.

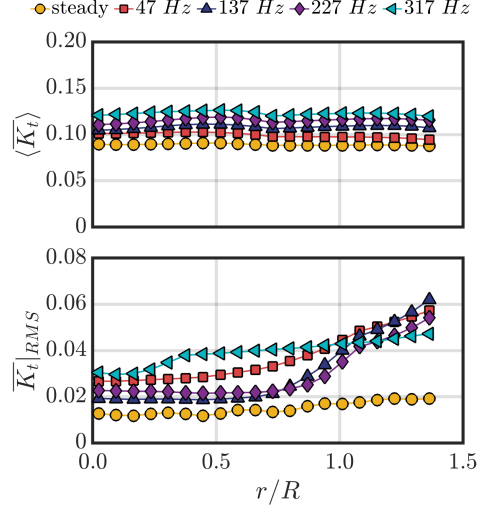

Figure 9: Radial profiles of mean and root-mean-square of normalized stretch rate due to tangential strain,  $\overline{K_t}$ , at different excitation frequencies and for the steady case of *constant power* method (markers are displayed every 3 data points for clarity).

### 2.3 Velocity and vorticity fields

Here, we show the mean ( $\langle \overline{V_z} \rangle$ ), and RMS ( $\overline{V_z}|_{RMS}$ ) of the normalized axial (streamwise) velocity ( $\overline{V_z} = V_z/U$ ) distribution, in columns (a) and (b) of Fig. 10, respectively. The strength of the vorticity, i.e., the mean of the square of the normalized vorticity ( $\langle \overline{\omega}^2 \rangle$ ) is shown in the columns (c) of Fig. 10. The results are shown for unsteady conditions at four excitation frequencies (rows i.–iv.) and for the steady (no oscillation) condition (row v).

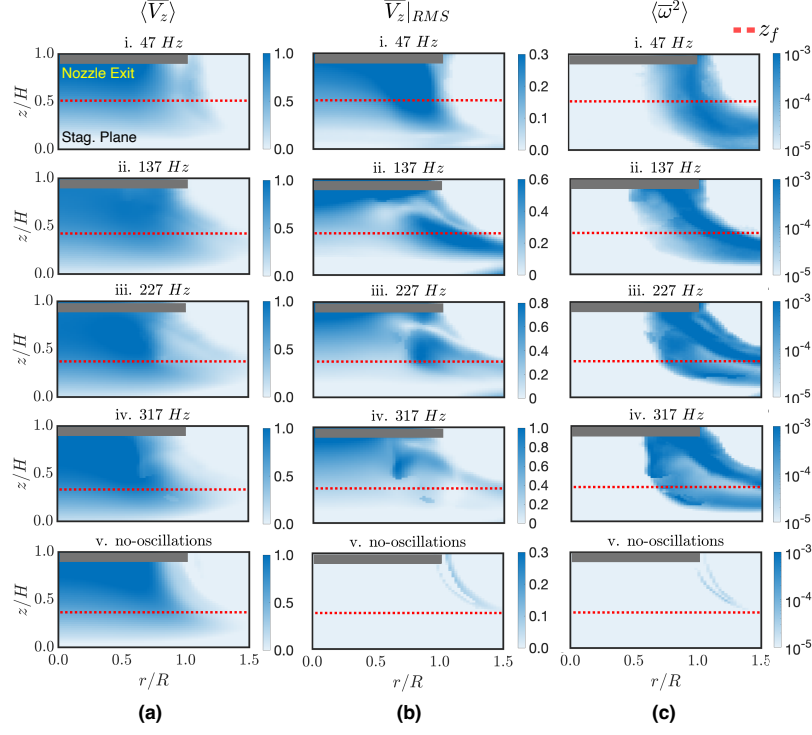

Figure 10: Color maps of *constant power* method for the distribution of (a) normalized stream wise mean velocity,  $\langle \overline{V_z} \rangle$ , (b) normalized stream wise root-mean-square velocity,  $\overline{V_z}|_{RMS}$ , and (c) normalized mean of vorticity squared,  $\langle \overline{\omega^2} \rangle$  at different excitation frequencies (i.) 47 Hz, (ii.) 137 Hz, (iii.) 227 Hz, and (iv.) 317 Hz, and for the steady (non-oscillated) case (v.). The mean flame location  $\langle z_f \rangle$  for each frequency case is depicted with a red dashed line. Color maps represent the field to the right of the counterflow vertical centerline and above the stagnation plane. The uncertainty in the computation of  $V_z$  is 0.01 – 0.02 m/s.

The phase-averaged vorticity field in Fig. 11 for  $f_e = 47$  Hz,  $f_e = 137$  Hz,  $f_e = 227$  Hz, and  $f_e = 317$  Hz. These phase-averaged snapshots spanning from  $\phi = 0^+$  to  $\phi = 2\pi^-$  reveal the real-time evolution and advection of the vortices along the shear layer. The sequence clearly shows the formation and advection of the pair of counter-rotating vortices ( $A_1$  and  $B_1$  in the figure) along the shear layer during the cycle, and their eventual approach towards the outer edge of the flame. The phase-averaged was computed similarly to the *constant amplitude* method.

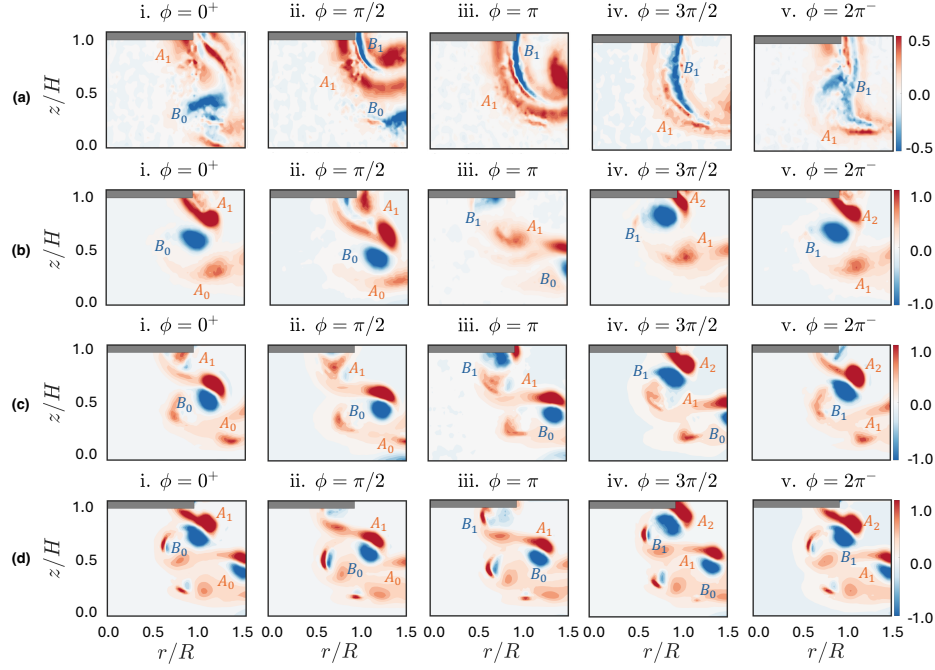

Figure 11: Phase-averaged vorticity for one excitation cycle for (a)  $f_e = 47$  Hz, (b)  $f_e = 137$  Hz, (c)  $f_e = 227$  Hz, and (d)  $f_e = 317$  Hz at five phase angles from  $0^+$  to  $2\pi^-$  (i-v.) of *constant power* method. The schematic represents the top-right quadrant corner of the counterflow. A and B are large counter-rotating vortex pairs generated during each cycle. Subscripts 0, 1, and 2 refer to vortices originating from the previous, current, and next cycle, respectively.

The power spectral density (PSD) of vorticity,  $\hat{P}_\omega$ , in the vicinity of the flame is shown next. Figure 12 compares  $\hat{P}_\omega$  at three radial locations. Along the centerline ( $r/R = 0$ ), which lies outside the shear layer, the vorticity spectrum is essentially flat across all frequencies (Fig. 12a), indicating negligible spectral energy. All these results are very similar to those of the *constant amplitude* method of excitation.

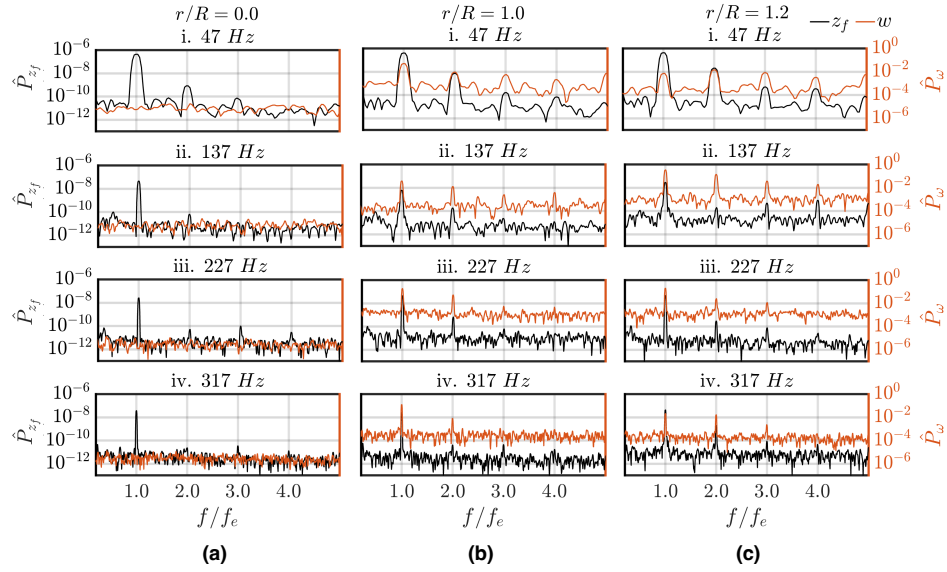

Figure 12: Power spectral density of flame displacement ( $\hat{P}_{z_f}$ ) and flow vorticity ( $\hat{P}_\omega$ ) measured at (a) center line ( $r/R = 0$ ), (b) flame location  $r/R = 1.0$ , and (c) flame location  $r/R = 1.2$  at different excitation frequencies ((i.) 47 Hz, (ii.) 137 Hz, (iii.) 227 Hz, and (iv.) 317 Hz) at mean flame location of *constant power* method.

### 3 Non-reactive vs. reactive data

To complement the cold-flow (or non-reactive) results presented in the main manuscript, we also examined the corresponding hot-flow (or reactive data). Below, we compare radial locations where 2nd harmonics become stronger, obtained from hot-flow and cold-flow data.

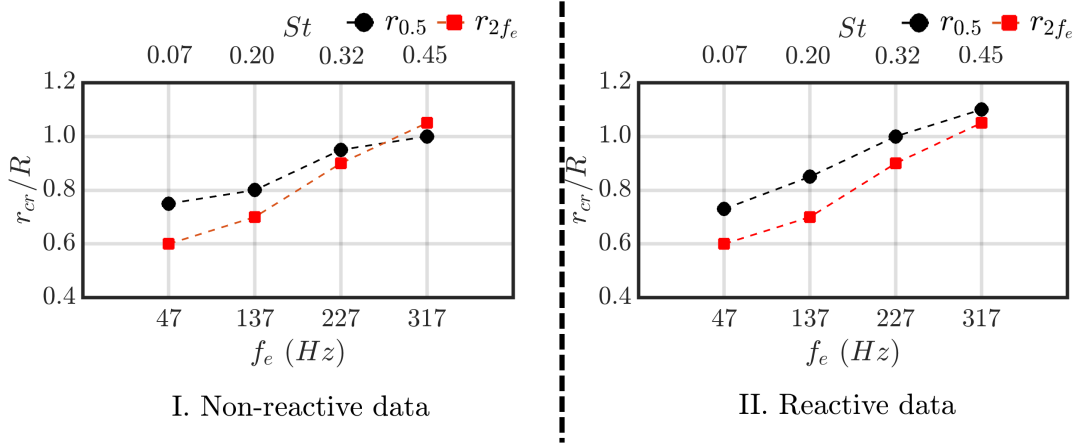

Figure 13: Comparison of I. Non-reactive data vs. II. Reactive data of the normalized critical radius where  $\langle \bar{\omega}^2 \rangle$  is 50% of its maximum, with normalized radial location where  $2f_e$  starts to increase in  $\hat{P}_{z_f}$  as a function of excitation frequency (shown in primary x-axis), and corresponding Stokes number,  $St = f_e t_F$  (shown in secondary x-axis).

Figure 13 compares  $r_{0.5}$  across the four excitation frequencies with the corresponding radial positions where the second harmonic ( $f/f_e = 2$ ) in flame oscillations begins to grow. The results confirm that the transition points of  $\langle \bar{\omega}^2 \rangle$  and the onset of second-harmonic growth in flame oscillations exhibit a consistent trend for both non-reactive and reactive data. It should be noted that alternative definitions of the transition radius (e.g., based on the maximum gradient or on 10% of the maximum value) also yield qualitatively similar trends.

## 4 Top flame vs. bottom flame

For completeness, we also include results from the local spectral signature of flame oscillation at both center and off-center locations for the bottom flame. Figure 7(a-c) presents the PSDs of the flame displacement ( $\hat{P}_{z_f(r)}$ ) at three radial locations: the centerline ( $r/R = 0$ ), and two off-center positions ( $r/R = 1.0$ , and  $r/R = 1.2$ ), for all four excitation frequencies comparing top flame (black) and bottom flame (red). The analysis shows that the same dynamics and trends observed in the top flame are reproduced in the bottom flame data. This consistency indicates that the underlying flame-flow interactions are symmetric with respect to the counterflow configuration, and that the conclusions drawn from the top flame analysis are representative of the overall system behavior.

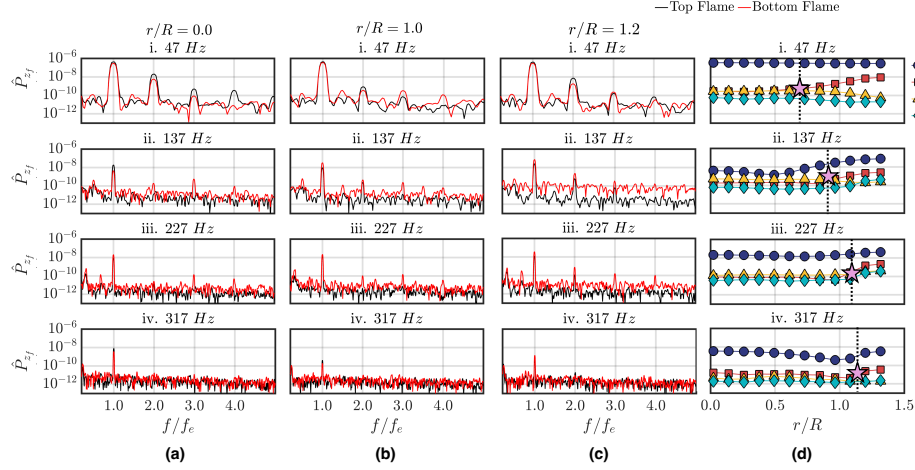

Figure 14: Power spectral density of bottom flame oscillation or displacement ( $\hat{P}_{z_f}$ ) measured at (a) flame's center point ( $r/R = 0$ ), (b) flame location  $r/R = 1.0$ , and (c) flame location  $r/R = 1.2$  accompanied by (d) radial profiles of first four harmonics of the  $\hat{P}_{z_f}$  (markers are displayed every 6 data points for clarity). The radial location ( $r_{2f_e}$ ) where  $2f_e$  starts to increase is marked with a star and a vertical dashed line in (d). Four rows represent four excitation frequencies: (i.) 47 Hz, (ii.) 137 Hz, (iii.) 227 Hz, and (iv.) 317 Hz.
